# Supplementary material for: Declarative Recursive Computation on an RDBMS, or, Why You Should Use a Database For Distributed Machine Learning
Source: arXiv:1904.11121 source file (2019-04-25)
Supplement: Supplementary file 1 [file appendix.tex]

%\renewcommand\appendixname{Appendix}
%\renewcommand\appendixpagename{Appendix}

%\clearpage
%\appendix
%\begin{appendices}

\section{Model Parallelism in TensorFlow}

It is instructive to take one of the most popular systems for deep learning and examine exactly what support it provides
for model parallelism.
That is, now might one implement a model parallel learner on such a system?  This is instructive for comparison with the 
declarative approach taken in this paper.
We now do exactly that for TensorFlow.

Imagine we have a four-layer, fully-connected feedforward neural network for the first learning problem considered in this
paper.  
As in this paper, the numbers of neurons for the input layer, the hidden layer one, the hidden layer two and the 
output layer are 60K, 40K, 40K and 17, respectively. We have a cluster of 10 machines, and 
want to train this neural network on this cluster in a model parallelism manner. 

The very first step is to partition the parameters of this neural net 
(e.g., the weight matrices and the error vectors) into a set of shards, and place those shards on the machines in the cluster. 
In TensorFlow, we can use the \texttt{partitioner} functionality
to distribute the weight matrices and the error vectors, 
and employ the built-in function \texttt{tf.train.replica\_device\_setter()} to place those shards across different machines. 

After partitioning the model, we can start training it by feeding it with number of mini-batches; 
for example, small subsamples of 100 data points from the main data set.  Imagine such a subsample is stored in 
matrix \textbf{X} with dimensions $100 \times 60$K.
The first computation conducted during training is the matrix-matrix multiplication $\mathbf{X \times W_{1}}$, 
where $\mathbf{W_{1}}$ is the weight matrix for the first layer, with dimensions $60$K $\times 40$K. 

Performing this matrix multiplication in TensorFlow is not trivial, 
given that $\mathbf{W_{1}}$ is partitioned and stored across a set of machines 
(and the matrix $\mathbf{X}$ may be partitioned as well when the number of data points is large). 
If we call the built-in function \texttt{tf.matmul} (which is the default function for the matrix multiply in TensorFlow) 
on the matrices $\mathbf{X}$ and $\mathbf{W_{1}}$, the system will fetch all pieces of $\mathbf{W_{1}}$ to one machine, and 
conduct the multiplication on that machine. For large matrices, this will fail.
Hence, we have to implement it ourselves. A typical implementation consists of four procedures: 
fetching the partitions of the matrix from different devices (using the function \texttt{tf.nn.embedding\_lookup}), 
doing a local matrix multiplication on those partitions, aggregating the results for the 
local multiplications, and storing the aggregated results in another partitioned matrix. It is also necessary to
embed in the code a specification of which devices to conduct those computations on.

%\end{appendices}
